# Supplementary material for: Efficient Estimation of Mutual Information for Strongly Dependent Variables
Source: arXiv:1411.2003 source file (2015-03-05)
Supplement: Supplementary file 5 [file mie_supplementary_old.tex]

\clearpage
\counterwithin{figure}{section}
\counterwithin{equation}{section}
\counterwithin{algorithm}{section}

\section*{Supplementary Material for ``Functional Relationship MIE''}


\section{Empirical Evaluation for $\alpha_{k,d}$}
\label{sec:derive_alpha}

Suppose a uniform distribution supported in the $d$ dimensional (hyper)rectangle with the volume $V$.  We sample $k$ points from this uniform distribution. After doing PCA on these $k$ points, we get the correcting volume $\bar V$. Because $k$ points are sampled from the uniform distribution, we always want to choose \textit{uniformity} not \textit{linearity} in this case. Thus, $\alpha_{k,d}$ must satisfy the following constraint:
\be\label{eq:alpha_1}
\Pr \left( {\frac{{\bar V}}{V} < {\alpha _{k,d}}} \right) = 0
\ee

Suppose we sample $k$ points for $N$ times, and get the volume $V_i$ and $\bar V_i$ for each time $i$. We can rewrite the Eq.~\ref{eq:alpha_1} as 
\be\label{eq:alpha_2}
\mathop {\lim }\limits_{N \to \infty } \frac{{\sum\limits_{i = 1}^N {{\bf{I}}\left( {\frac{{\bar {{V_i}}}}{{{V_i}}} < {\alpha _{k,d}}} \right)} }}{N} = 0
\ee
where $\bf{I}(\bullet)$ is the indicator function taking two values in $\{0,1\}$. 

For any $\alpha_{k,d}$ that satisfies Eq.~\ref{eq:alpha_1} or Eq.~\ref{eq:alpha_2}, we have the following Theorem \note{which can be easily proved?}
\be
\mathop {\lim }\limits_{M \to \infty } {\widehat I_{LNC}}\left( \vx \right) \equiv {\widehat I_{KSG}}\left( \vx \right)
\ee
where $M$ is the number of samples from random variable $\vx$.

Obviously, any $\alpha_{k,d} \le 0$ can satisfy Eq.~\ref{eq:alpha_2} but this will lead to no correction happen. Therefore, we really want to find the max value that satisfies Eq.~\ref{eq:alpha_2}, i.e., 
\be
\begin{array}{l}
{\alpha _{k,d}} = \max \left( \alpha  \right)\\
s.t.\mathop {\lim }\limits_{N \to \infty } \frac{{\sum\limits_{i = 1}^N {{\bf{I}}\left( {\frac{{\bar {{V_i}}}}{{{V_i}}} < \alpha } \right)} }}{N} = 0
\end{array}
\ee

This optimization problem is hard to solve because the distribution of ${\frac{{\bar {{V}}}}{{{V}}}}$ is unknown. However, we can estimate $\alpha_{k,d}$ empirically. We choose a large $N$ and $\hat \alpha_{k,d}$ such that $\sum\limits_{i = 1}^N {{\bf{I}}\left( {\frac{{\bar {{V_i}}}}{{{V_i}}} < {{\hat \alpha }_{k,d}}} \right)} /N < \epsilon $ where $\epsilon$ is a relatively small value\footnote{In practice, we choose $\epsilon = 5\times10^{-3}$ and $N = 5\times{10^5}$}.  The following algorithm describes this procedure:

\begin{algorithm}[h]
\caption{\textbf{Estimating $\alpha_{k,d}$ for LNC}}
\begin{algorithmic}
\label{alg:alpha}
\State{\textbf{Input:} parameter $d$ (dimension), $k$ (nearest neighbor), $N$, $\epsilon$}
\State{\textbf{Output:} $\hat \alpha_{k,d}$}

\State{set array $\bf{a}$ to be NULL}
\Repeat
	\State{Randomly choose a uniform distribution supported on $d$ dimensional (hyper) rectangle, denote its volume to be $V$}
	\State{Draw $k$ points from this uniform distribution, get the correcting volume $\bar V$ after doing PCA}
	\State{add the ratio $\frac{\bar V}{V}$ to array $\bf{a}$}
\Until above procedure repeated $N$ times

\State{$\hat \alpha_{k,d} \leftarrow \left\lceil\epsilon N\right\rceil th$ smallest number in $\bf{a}$}
\end{algorithmic}
\end{algorithm}

\newpage 
Figure~\ref{fig:alpha} shows empirical value of $\hat \alpha_{k,d}$ for different $(k,d)$ pairs. We can see that for a fixed dimension $d$, $\hat \alpha_{k,d}$ grows as $k$ increases, meaning that $\bar V$ must be closer to $V$ to accept a \textit{Uniformity} hypothesis as number of points $k$ becomes larger.

Furthermore, we also find that $\hat \alpha_{k,d}$ decreases as the dimension $d$ increases, indicating that for a fixed $k$, $\bar V$ becomes much smaller than $V$ given a uniform distribution in higher dimensions.

\begin{figure}[htbp]
	\centering
	\includegraphics[width=0.5\textwidth]{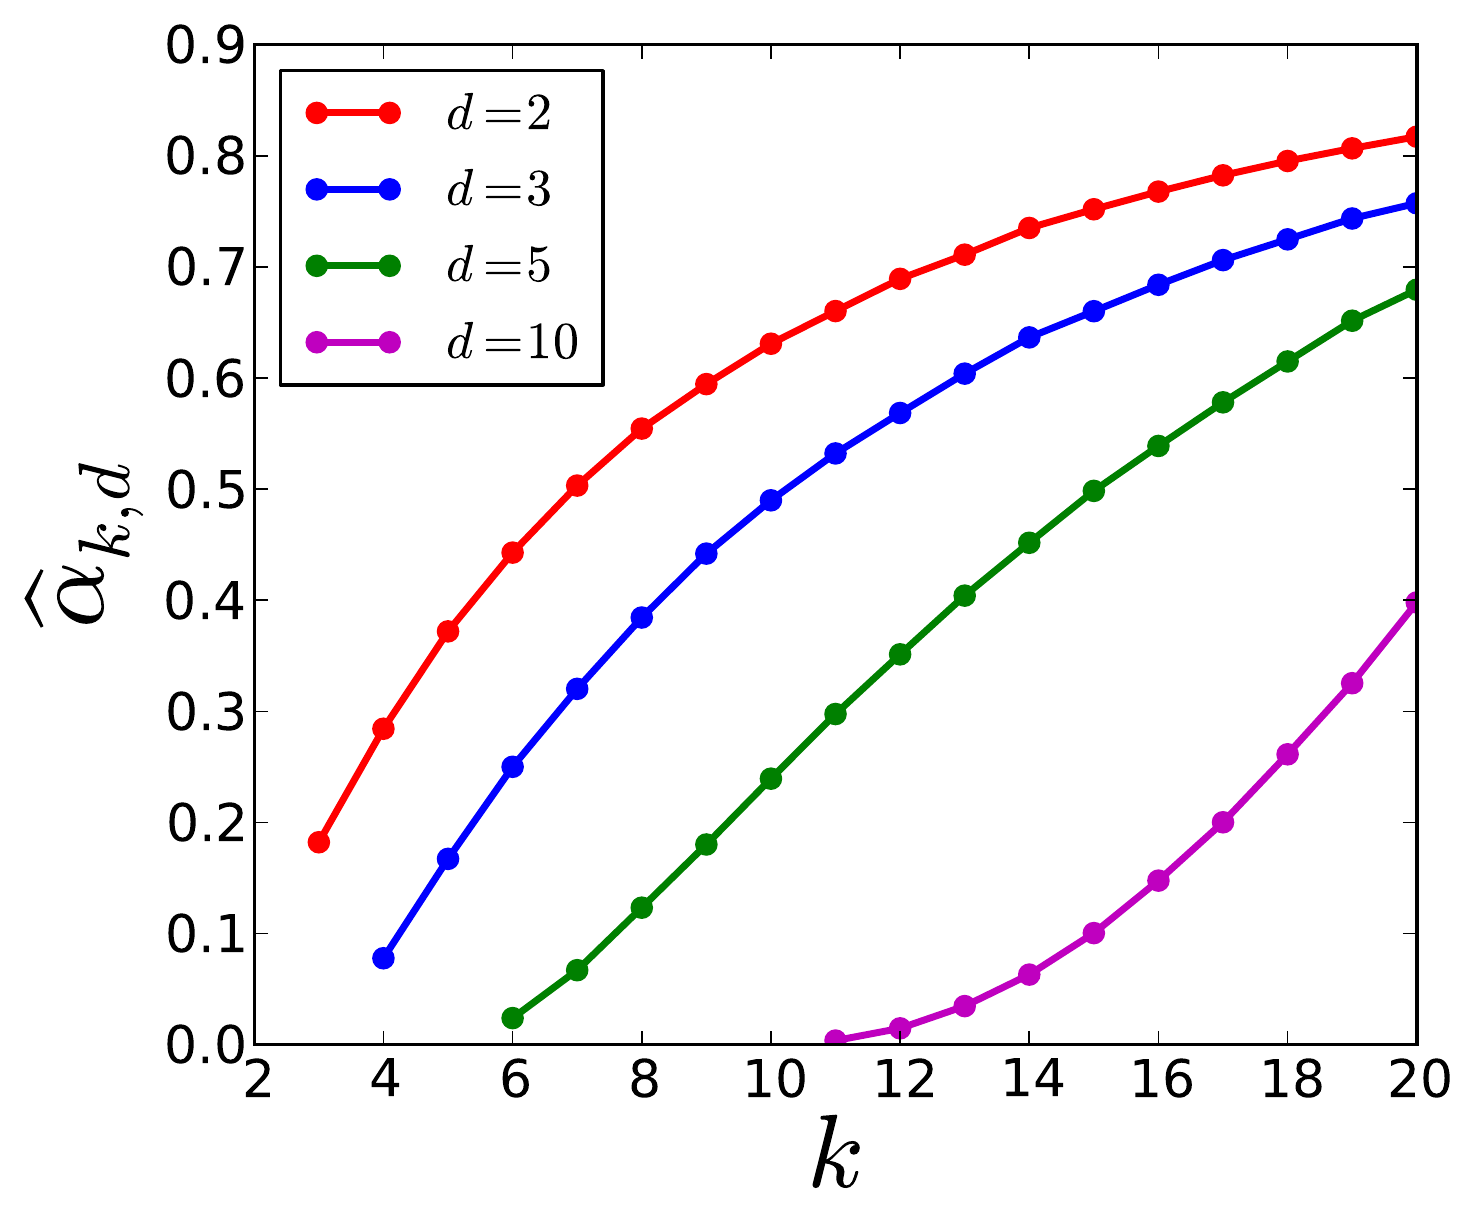}
	\caption{$\widehat \alpha_{k,d}$ as a function of $k$. $k$ ranges over $[d,20]$ for each dimension $d$.}
	\label{fig:alpha}
\end{figure}


\section{More Functional Relationship Tests in Two Dimensions}
We have tested together twenty-one functional relationships described in Kinney and Atwal's paper\footnote{Reshef's paper~\cite{reshef} also tests these functions.}~\cite{kinney}, we show six of them in Section~\ref{sec:func}. Here all the results are illustrated in Figure~\ref{fig:all_functions}. Detailed description of the functions can be found in Table S1 of Supporting Information in~\cite{kinney}. 

\begin{sidewaysfigure}[ht]
    \includegraphics[width=1.1 \columnwidth]{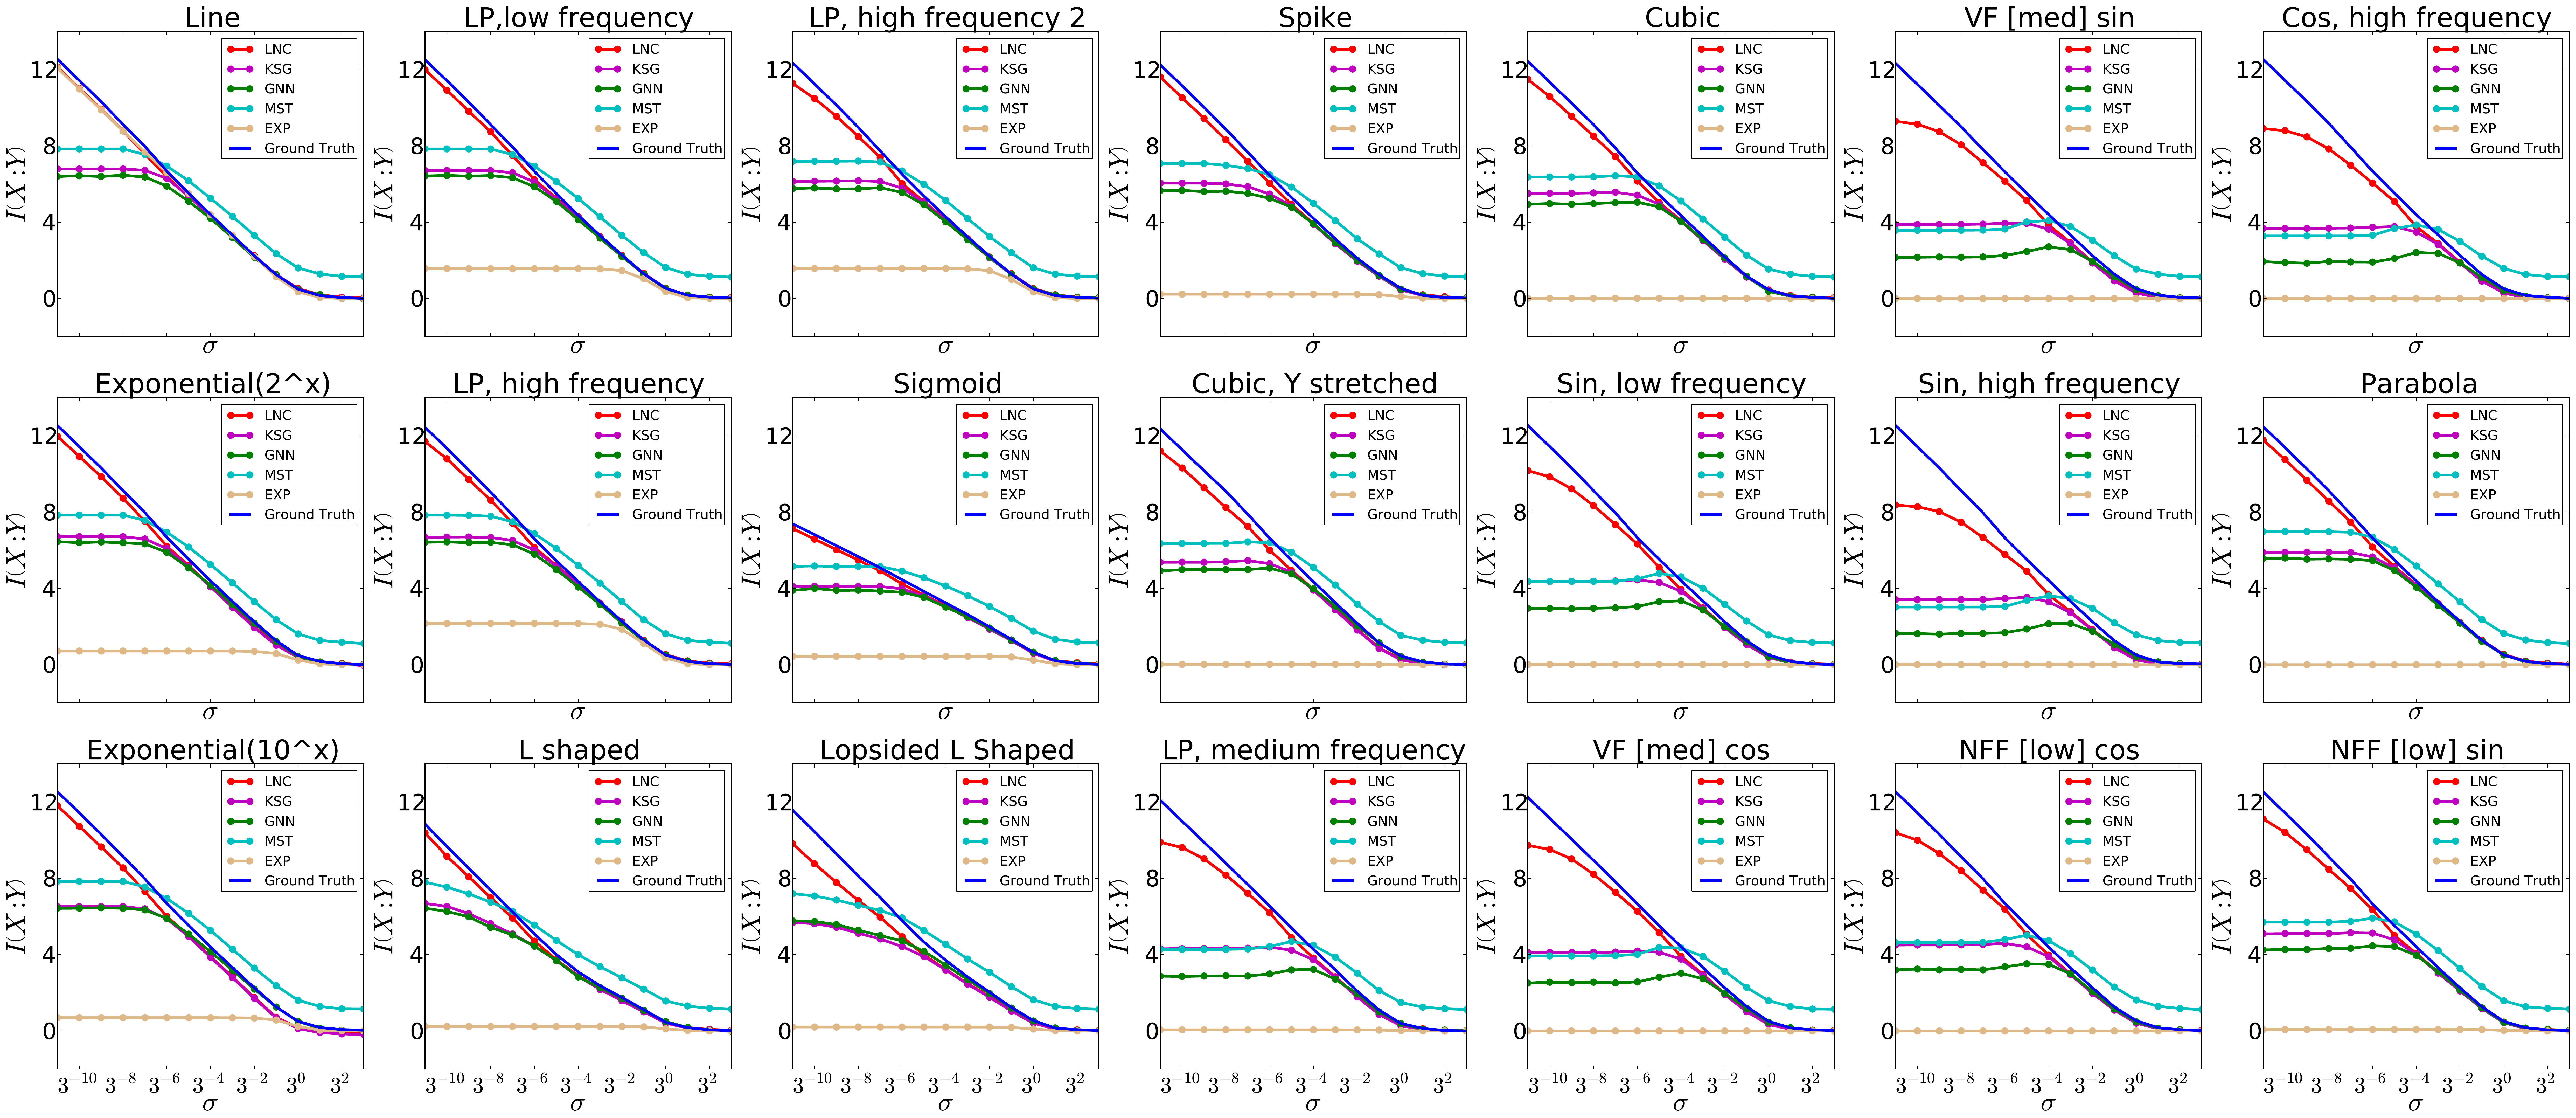}
    \caption{Mutual Information tests of $LNC$, $KSG$, $GNN$, $MST$, $EXP$ estimators. Twenty-one functional relationships with different noise intensities are tested. Noise has the form $U[-\sigma/2,\sigma/2]$where $\sigma$ varies(as shown in X axis of the plots). For KSG, GNN and LNC estimators, nearest neighbor parameter $k=5$. We are using $N = 5,000$ data points for each noisy functional relationship.}
    \label{fig:all_functions}
\end{sidewaysfigure}
